# Supplementary material for: Conditional Disclosure as a Coordination Device
Source: arXiv:2604.00874 source file (2026-10-09)
Supplement: Supplementary file 1 [file conditional_disclosure_online_appendix.tex]

\documentclass[conditional_disclosure.tex]{subfiles}

\begin{document}

\ifSubfilesClassLoaded{%
  \title{Supplemental Appendix\\Conditional Disclosure as a Coordination Device}
  \shortTitle{Supplemental Appendix: Conditional Disclosure}
  \issueName{}
  \ifanonymizeforpeerreview
    \author{Anonymous}
  \else
    \author{Matthew Cashman\thanks{Cashman: MIT Sloan School of Management, cashman@mit.edu.}}
  \fi
  \date{}
  \begin{abstract}
  \end{abstract}
  \maketitle
}{ }

\startsupplement

\ifSubfilesClassLoaded{ }{%
  \appendixparttitle{Supplemental Appendix}
}

This Supplemental Appendix develops three parts of the argument that are useful but not needed for the article's central comparison. First, it replaces the continuum with a literal finite group and shows how a common signing cutoff works when one person can affect publication. Second, it distinguishes hiding a failed signer list from hiding the fact that a campaign was attempted, and explains when coalition size summarizes all the information in a named list. Third, it describes how existing institutional and cryptographic tools can implement conditional disclosure. The article contains the continuum selection proof and common-rank accounting result.

\section{Appendix B. Finite Committed-Core Benchmark}\label{app:finite_core}

This section replaces the continuum of the article with a literal group of $N$ marginal agents. Unlike an infinitesimal agent in the continuum, each of these people contributes one whole signature and may be pivotal: adding her name can move the final count across the threshold. The section asks whether a simple cutoff rule remains meaningful when each person has this positive chance of affecting publication and does not know how many others will sign.

Let the state $\theta$ measure the underlying favorability of the environment. It lies in $[\underline\theta,\overline\theta]$. Before receiving private information, agents share a prior density $g$, which assigns positive probability density continuously across that range and describes how plausible they initially find each state. The integer publication threshold satisfies $K\ge2$. A weakly increasing measurable function
\begin{equation}
B:[\underline\theta,\overline\theta]\longrightarrow\{0,1,\ldots,K\}
\end{equation}
gives the number of committed or protected signers in each state. Thus $B(\theta)$ is a count, not a probability. These core signers participate independently of the marginal agents' decisions. The remaining $N$ agents decide simultaneously whether to join the list. Because $B$ is weakly increasing, more favorable states have at least as many committed signers as less favorable states.

The function $B$ and the prior are common knowledge, but the realized state and hence the realized core count $B(\theta)$ are not observed before marginal agents act. During the simultaneous collection period, each marginal agent observes only her own signal: she does not observe other signals, other marginal decisions, or an interim count.

Agent $i$ observes
\begin{equation}
x_i=\theta+\sigma\varepsilon_i,
\end{equation}
where $\sigma>0$ controls signal noise. The shocks $\varepsilon_i$ are independent across agents, independent of $\theta$, and identically distributed with continuous strictly increasing distribution $F$ and positive density $f$; the structure satisfies monotone likelihood ratios. If agent $i$ signs and $Q_{-i}$ other marginal agents sign, publication occurs when
\begin{equation}
B(\theta)+1+Q_{-i}\ge K.
\end{equation}
Successful publication gives the signer the private value $v(x_i)\ge0$ of being named on the released list, where $v$ is continuous and strictly increasing. A non-signer receives no expressive or substantive payoff from another coalition's publication. This normalization keeps the decision focused on the private return from joining; a public benefit enjoyed by non-signers would add a separate motive to be the person whose signature causes publication. Signing costs $k>0$ whether or not publication occurs. Ideal failure privacy gives no expressive value or exposure payoff after failure, so signing yields
\begin{equation}
u_i(1,Q_{-i},\theta;x_i,k)
=\ind\{B(\theta)+1+Q_{-i}\ge K\}v(x_i)-k,
\end{equation}
whereas not signing yields zero. The agent pays $k$ for certain and receives $v(x_i)$ only if the list is published.

A symmetric cutoff $s$ has every marginal agent sign exactly when her signal is at least $s$; by convention, equality leads to signing. Allowing $s\in\overline{\mathbb R}=\mathbb R\cup\{-\infty,+\infty\}$ includes the extreme rules ``always sign'' and ``never sign.'' Under this conjecture, another marginal agent signs in state $\theta$ with probability
\begin{equation}
p_s(\theta)
=1-F\!\left(\frac{s-\theta}{\sigma}\right).
\end{equation}
Use the conventions $p_{-\infty}=1$ and $p_{+\infty}=0$.
Conditional on $\theta$, each of the other $N-1$ agents independently signs with this probability, so their total is $Q_{-i}(s)\sim\operatorname{Binomial}(N-1,p_s(\theta))$. After observing $x$, agent $i$ holds the posterior density
\begin{equation}
g(\theta\mid x)
=\frac{g(\theta)f((x-\theta)/\sigma)}
{\int_{\underline\theta}^{\overline\theta}g(t)f((x-t)/\sigma)\,dt}.
\end{equation}
For a given state, define $r(\theta)=\max\{0,K-B(\theta)-1\}$ as the minimum number of other marginal signers needed for publication after agent $i$ joins. The state-contingent success probability is the upper tail of the binomial distribution:
\begin{equation}
\begin{aligned}
\pi(\theta;s)
&=\sum_{q=r(\theta)}^{N-1}
\binom{N-1}{q}p_s(\theta)^q\{1-p_s(\theta)\}^{N-1-q},\\
r(\theta)&=\max\{0,K-B(\theta)-1\},
\end{aligned}
\end{equation}
with the sum interpreted as zero if $r(\theta)>N-1$. The success probability conditional on agent $i$'s signal is then derived from primitives as
\begin{equation}
\Pi(x;s)
=\int_{\underline\theta}^{\overline\theta}
\pi(\theta;s)g(\theta\mid x)\,d\theta.
\end{equation}
The function $\pi(\theta;s)$ answers: if the true state were known to be $\theta$, how likely would the contract be to publish after agent $i$ signs? The function $\Pi(x;s)$ averages that probability over the states the agent considers possible after seeing signal $x$. Because both the core $B(\theta)$ and each opponent's signing probability $p_s(\theta)$ rise with the state, $\pi(\theta;s)$ is weakly increasing. Monotone likelihood ratios make the posterior more favorable as $x$ rises, so $\Pi(x;s)$ is weakly increasing in $x$. A signer's expected payoff is therefore
\begin{equation}
V(x;s,k)=\Pi(x;s)v(x)-k.
\end{equation}
This expression has a direct interpretation: probability of publication times value conditional on publication, minus the signing cost.

The following regularity assumption makes best responses and equilibrium cutoffs well behaved. It requires clear low- and high-signal dominance regions, a unique signal at which an agent is indifferent when everyone uses the same cutoff, and no reversals in the sign of that indifference condition.

\begin{assumption}[Finite symmetric-cutoff regularity]\label{ass:finite_core_selection}
There are nonempty low- and high-state intervals on which $B(\theta)+N<K$ and $B(\theta)\ge K$, respectively. The first condition implies $N<K$: the model describes a marginal fringe that cannot publish without some core participation, while the core can publish by itself in favorable states. For each cutoff $s\in\overline{\mathbb R}$, $\Pi(x;s)$ is jointly continuous in $(x,s)$ and $V(\cdot;s,k)$ is continuous and strictly increasing on the relevant signal interval. Uniformly over $s\in\overline{\mathbb R}$ and $k$ in the compact interval $\mathcal K\subset(0,\infty)$, there are signals $x_L<x_H$ such that $V(x_L;s,k)<0<V(x_H;s,k)$. For every $k\in\mathcal K$, the diagonal payoff
\begin{equation}
\Phi_k(s)\equiv V(s;s,k)
\end{equation}
is continuous, has a unique root $s^*(k)$, and satisfies $\Phi_k(s)<0$ for $s<s^*(k)$ and $\Phi_k(s)>0$ for $s>s^*(k)$.
\end{assumption}

The prior and signal structure generate $\Pi$ and ensure that a better signal does not lower the chance of success. The remaining conditions in Assumption~\ref{ass:finite_core_selection} control the feedback between one agent's decision and what she expects others to do. The diagonal payoff $\Phi_k(s)=V(s;s,k)$ evaluates an agent whose signal is exactly $s$ when she expects every other marginal agent to use that same cutoff. A root of $\Phi_k$ is therefore a self-consistent boundary: the agent at the boundary is indifferent, agents above it prefer to sign, and agents below it prefer not to sign. The assumption requires this boundary to be unique and rules out a payoff that crosses zero, reverses direction, and crosses again. The prior and the existence of a core do not by themselves guarantee these properties. Uniform dominance, a strictly increasing best response, and the unique diagonal crossing are maintained regularity conditions. They play the same formal role as diagonal-crossing restrictions in monotone global-games selection arguments \citep{frankelEquilibriumSelectionGlobal2003}.

\begin{proposition}[Finite cutoff characterization]\label{prop:finite_core_selection}
Under Assumption~\ref{ass:finite_core_selection}, the finite marginal-agent game has a unique symmetric monotone cutoff value. Under the maintained boundary convention, marginal agent $i$ signs if and only if $x_i\ge s^*(k)$. Without that convention, cutoff strategies may differ only in the action assigned to the indifferent, zero-probability boundary signal. If $k_2>k_1$ are in $\mathcal K$, then $s^*(k_2)>s^*(k_1)$. Consequently, for every state $\theta$,
\begin{equation}
\begin{aligned}
&\Prob\!\left(B(\theta)+Q_N(s^*(k_2))\ge K\mid\theta\right)\\
&\qquad\le
\Prob\!\left(B(\theta)+Q_N(s^*(k_1))\ge K\mid\theta\right).
\end{aligned}
\end{equation}
\end{proposition}

The proposition has two economic conclusions. Within symmetric monotone strategies, agents sign when their signals exceed one common cutoff. A higher signing cost raises that cutoff, so a stronger signal is needed to make signing worthwhile. Fewer agents then sign, and the probability of publication cannot increase in any state. This finite result concerns participation and publication within the contract. It does not compare the contract with open expression or model how a signer's exposure changes with coalition size, so it does not prove the article's exposure-tail result for a finite population.

\begin{proof}
For any conjectured cutoff $s$, continuity, strict increase, and the uniform low- and high-signal inequalities make the best response another finite cutoff. The agent at its boundary is indifferent. In a symmetric monotone cutoff equilibrium, the conjectured cutoff and the best-response cutoff must be the same, so the marginal signal satisfies $V(s;s,k)=0$. Assumption~\ref{ass:finite_core_selection} gives the unique solution $s^*(k)$, and the weak-inequality convention says that the indifferent boundary agent signs. The proposition does not claim uniqueness among asymmetric or nonmonotone equilibria. It also assumes, rather than derives from the primitive prior and signal structure, that the diagonal payoff has a unique crossing.

Set $s_1=s^*(k_1)$. Since $k_2>k_1$,
\begin{equation}
\Phi_{k_2}(s_1)=\Phi_{k_1}(s_1)-(k_2-k_1)<0.
\end{equation}
The global sign pattern for $\Phi_{k_2}$ implies $s^*(k_2)>s_1$. Raising the cutoff weakly lowers the number of marginal signers for every realized collection of private signals. The total $B(\theta)+Q_N$ therefore falls \emph{pathwise}: for each possible realization, not merely on average. An event that was below threshold cannot become successful when the cutoff rises, which gives the state-by-state publication-probability inequality.
\end{proof}

\section{Appendix C. Failed-List Privacy, Attempt Observability, and Exchangeability}\label{app:privacy_exchangeability}

Failure privacy contains two distinct informational restrictions that are easy to conflate. First, a failed contract does not disclose its signer list or count. Second, treating failure as a public non-event requires the campaign attempt itself to be unobserved by the outside audience whose reaction generates exposure costs. A mechanism can satisfy the first restriction without satisfying the second. In the ideal benchmark, that audience observes
\begin{equation}
o=
\begin{cases}
\mathcal{C}, & q\ge\tau,\\
\varnothing, & q<\tau,
\end{cases}
\end{equation}
where $\mathcal{C}$ is the successful named coalition and $\varnothing$ means that the audience sees no list, count, failure announcement, or other indication that a campaign was attempted. Eligible agents may know that they received an offer and may infer after the deadline that publication did not occur. That private inference neither identifies other signers nor creates a public signal for the exposure-cost audience.

If the campaign's existence is publicly observable, a missing publication is an observed failed attempt rather than the public non-event represented by $\varnothing$. Failed-list privacy still protects names, but the audience can revise its beliefs after learning that a campaign was tried and fell short. Public attempt observability therefore defines a second information regime. A data breach or premature release is different: it exposes information that the promised rule was supposed to withhold.

The article also uses an exchangeability assumption to summarize a published coalition by its size: seeing Alice, Bob, and Carol rather than three other eligible people conveys no information beyond seeing a coalition of size three, so coalition size is a sufficient statistic for public inference.

\begin{lemma}[Exchangeable identities]\label{lem:exchangeable_identities}
Suppose that, conditional on the state and the symmetric strategy, all coalitions of a given size have the same likelihood, and that identities carry no payoff-relevant public covariates beyond coalition membership. If publication reveals a named coalition $\mathcal{C}$, then coalition size is sufficient for public inference:
\begin{equation}
\Prob(\theta\mid \mathcal{C},\mathrm{publication})
=
\Prob(\theta\mid |\mathcal{C}|,\mathrm{publication}).
\end{equation}
If $\mu(y)$ denotes the resulting audience belief at coalition size $y$, signer exposure costs may consequently be represented as
\begin{equation}
c_i(\mathcal{C})=\alpha_i\ell\bigl(|\mathcal{C}|,\mu(|\mathcal{C}|)\bigr).
\end{equation}
\end{lemma}

\begin{proof}
Under the stated exchangeability condition, the likelihood of a particular published coalition $\mathcal{C}$ depends on the state only through its size $|\mathcal{C}|$. Bayes' rule therefore gives the same state posterior for every coalition of that size. The cost representation follows from the additional restriction that audience response depends on the coalition only through its size and the induced belief.
\end{proof}

Lemma~\ref{lem:exchangeable_identities} says when coalition size contains all the information that the audience learns from the identities on a published list. It does not show that the article's selection theorem continues to hold when the audience changes its beliefs as the coalition grows. That theorem holds $\mu$ fixed so that a larger coalition affects exposure directly through safety in numbers, not indirectly through a changing audience inference. If audience beliefs are instead written as $\mu(y)$, effective exposure becomes $\ell(y,\mu(y))$. Coalition size then works through both channels at once. Applying the theorem would require this combined function to remain bounded, continuous, and strictly decreasing, and would also require the dominance and single-crossing conditions to continue to hold. Exchangeability alone provides none of these additional properties. The appendix therefore makes no general selection claim for an audience whose response changes with coalition size.

Names still determine which agents become publicly associated with the statement and therefore who bears exposure. Exchangeability removes composition effects among coalitions of the same size. When signer attributes affect public inference, protection, or retaliation, coalition composition becomes an additional payoff-relevant state variable.

\section{Appendix D. Implementation with Existing Tools}\label{app:implementation}

A fixed-population social assurance contract requires four operational functions. It must verify that each eligible person submits at most one endorsement, keep names and signatures confidential during collection, determine whether the threshold has been met, and release the complete authenticated list only after success. Existing cryptographic systems already perform close versions of each function. A proof-of-concept threshold secret petition accepts encrypted signatures from validated users, prevents duplicate signatures, divides decryption control among trustees, and makes the signatures readable after the threshold is reached \citep{breuerSeCritMassThresholdSecret2024}. Secure allegation escrows divide confidential allegations and identities among independent parties and reveal them after designated matching thresholds are reached; these systems include formal security analyses and prototype implementations \citep{arunFindingSafetyNumbers2020}. \citet*{mangipudiCollusionDeterrentThresholdInformation2023} develop a related threshold information escrow that deters trustee collusion. Each required function therefore has a close precedent. None of the cited systems implements and evaluates the exact combination described below under one set of assumptions about possible attacks and failures. A production system would still need to integrate the components, undergo a security audit and usability testing, and operate under clear governance rules.

\subsection{A Feasible Architecture}\label{app:implementation_architecture}

The least technical implementation delegates every function to an independent custodian such as a law firm, regulator, union, or ombudsperson. The custodian verifies participants against a roster, stores the list under access controls, and follows an audited release and destruction rule. Professional duties, contractual penalties, independent audits, and reputational capital can make this arrangement credible using ordinary institutional tools. Its tradeoff is concentrated trust: one organization can inspect, alter, suppress, or prematurely disclose the list.

When that concentration of trust is unacceptable, an alternative design separates five jobs. The \emph{sponsor} fixes the contract but never receives submissions. A \emph{registrar} verifies real-world eligibility. A \emph{collection service} checks and counts encrypted submissions. An independent \emph{auditor} resolves disputes about whether a valid submission was included. Finally, $m$ independent \emph{trustees} control whether submissions can be opened. The trustees jointly generate an encryption key used only for that campaign, and each retains only one share of it; no central operator ever possesses the complete key. At least $t$ trustees must cooperate to reconstruct the power to decrypt, where $1<t\le m$. Existing institutions could fill these roles. Assigning the jobs to different institutions avoids giving one actor both the identities and the power to release the list.

Each cryptographic tool has a distinct job. A digital signature is the electronic counterpart of signing a particular document: it proves that the holder of a particular key endorsed an exact statement and that the statement has not since changed. Encryption turns the signed record into unreadable ciphertext. Threshold decryption divides the power to reverse that encryption among several trustees, so no trustee can reveal a record alone. A zero-knowledge proof lets the collector verify a fact about the encrypted record---for example, that it contains an eligible identity and a valid signature---without learning the hidden identity or signature. These tools answer different questions: authenticity, secrecy, shared release control, and verification without disclosure.

\begin{enumerate}
\item Before recruitment, the sponsor fixes the exact statement, an objectively verifiable eligibility roster or rule, the endorsement threshold $K_N$, the closing time, and the success and failure disclosures. It also fixes any cancellation and emergency rules. A digital signature records assent to those terms; encryption makes the signed record unreadable during collection. Neither tool substitutes for the other.

\item The registrar verifies each member of $\mathcal{I}_N$ once and issues a cryptographically verifiable eligibility credential. The credential certifies either her identity or a public signing key that only she controls and that the registrar has linked to her identity. Registration can occur before any campaign so that approaching the registrar does not itself reveal an intent to sign. An anonymous credential lets a person prove eligibility to the collector without identifying herself at that stage; established systems also support one-use credentials and later opening under stated conditions \citep{camenischEfficientSystemNontransferable2001}.

\item A participant signs the exact statement and a unique identifier for this contract with her identity-bound key. She submits an encrypted record containing that signature, her certified identity, and the identifier. She also submits a campaign-specific serial number and a zero-knowledge proof, which is evidence about hidden information that does not reveal the information itself. The proof establishes that the encrypted identity or key is the one certified by the registrar and that the record contains a valid signature on this contract. Anonymous-credential and private-contract systems supply the component proof techniques for these checks \citep{camenischEfficientSystemNontransferable2001,kosbaHawkBlockchainModel2016}. The credential always produces the same serial number when used twice in this campaign but produces an unrelated number in a different campaign. The collector can therefore detect a second use without learning the participant's identity or linking her actions across campaigns. Coconut implements this eligibility and duplicate-prevention pattern in an electronic-petition application \citep{sonninoCoconutThresholdIssuance2019}.

\item The collection service verifies the proof, rejects a repeated serial number, and records each accepted encrypted submission in a private authenticated log. Authentication makes later deletion or alteration detectable. The service returns a signed inclusion receipt. A participant who receives no receipt, or whose receipt is omitted from the count, can challenge the omission privately before an independent auditor. This makes suppression contestable without publishing a failed participant's name or action.

\item The committed core uses the same authenticated submission process, and its accepted submissions count toward $K_N$. Core participation is independent of the marginal participants' choices. Consistent with the finite benchmark, the service reveals no interim core or total count to marginal participants. At the deadline, the collector and trustees audit the accepted log. If no operator should learn the count, secure multiparty computation can test whether private inputs reach $K_N$ without giving all inputs to one party \citep{evansPragmaticIntroductionSecure2018}.

\item At the preannounced close, each trustee verifies the integrity and count of the same private accepted log, and the auditor resolves any timely challenge backed by an inclusion receipt. If the accepted count reaches $K_N$, at least $t$ trustees sign a success certificate binding together the contract identifier, deadline, final count, and a cryptographic fingerprint of the exact accepted ciphertext set. A cryptographic fingerprint is a short value that changes if that set is altered, so the certificate identifies the precise encrypted records the trustees approved. The same quorum then combines its decryption-key shares. The resulting publication contains every accepted identity and signature, and any reader can verify both the registrar's identity binding and the participant's signature on the contract. The endorsement threshold $K_N$ and trustee quorum $t$ are different parameters: the first determines whether publication is authorized; the second determines how many custodians must cooperate to make the records readable. If the count falls short, the institution publishes nothing, the collector deletes the identity-bearing records, and the trustees erase the campaign-specific key shares. Failure privacy assumes that fewer than $t$ trustees collude before that erasure and that a later coalition of $t$ trustees has not retained copies of its shares.
\end{enumerate}

This reference workflow creates no public transaction, log entry, or counter for an individual submission, and it issues no public failure notice. Only success produces a public certificate and named list. It matches the article's failure observation $\varnothing$ only if network traffic and recruitment also conceal the attempt from the audience that could punish signers. The requirements for hiding those traces are discussed below.

Several familiar technologies can replace parts of this workflow. Threshold cryptography divides decryption control so that no one trustee can open a record, while a specified quorum can combine its shares. Secure allegation escrows demonstrate distributed conditional revelation \citep{arunFindingSafetyNumbers2020}, and \citet*{mangipudiCollusionDeterrentThresholdInformation2023} show how to deter premature trustee collusion. A smart contract is program code that a blockchain executes and records according to precommitted rules. Privacy-preserving voting systems show that such contracts can enforce eligibility, proof checks, stages, and tallying for a fixed group \citep{mccorrySmartContractBoardroom2017}. More general systems use encrypted information and zero-knowledge proofs to enforce private contract logic without placing the underlying information in clear text on a public ledger \citep{kosbaHawkBlockchainModel2016}.

\paragraph{Public-counter variant}
A public ledger is a replicated record that many computers maintain and that is designed to make past entries hard to alter. It can hold encrypted records or cryptographic fingerprints of them. Encryption can keep record contents secret, and fingerprints make alteration detectable. A fingerprint does not contain the underlying record, however, so copies stored elsewhere are still needed to ensure \emph{availability}: the ability to retrieve the record when authorized. Public per-submission records also reveal that a campaign exists and may reveal its running count. Such a design implements failed-name privacy, but not the article's stronger public non-event unless both submission traffic and the count are hidden through fixed-size batches, decoy traffic, or another privacy layer. Putting identity-bearing ciphertexts on an immutable ledger also leaves permanent encrypted material that a future key compromise could expose. For the benchmark-compatible workflow, those ciphertexts therefore remain off the public ledger; a ledger may instead record the precommitted terms and, after success, the certificate and released list. Any public-ledger variant additionally relies on the security and availability of its consensus system, the rules by which participating computers agree on the ledger's valid state.

Separating these roles limits what any one actor can learn or do. The registrar can know who is eligible without learning who submitted. The collector can verify that submissions are unique without reading them, and no single trustee can open a failed list. The sponsor cannot change the statement or threshold after observing participation. Submission receipts let a private auditor detect omitted entries or cases in which the collector showed different participants different versions of the log. No component eliminates the need for reliable operation. The design still assumes that credentials are issued correctly or audited, participant devices and software work as intended, and all trustees use the same log. It also requires at least $t$ trustees to remain available after success, fewer than $t$ trustees to collude before success, and key shares to be erased after failure. Engineering controls, audits, and governance rules can support these conditions, but they must be evaluated for each deployment.

\subsection{Threats and Mitigations}\label{app:implementation_threats}

\paragraph{Eligibility and malicious participation}
A Sybil attack occurs when one actor presents several identities and is therefore counted several times \citep{douceurSybilAttack2002}. A fixed eligibility roster makes this problem much easier than proving that every account on the open internet belongs to a different person. The sponsor freezes the roster rule, the registrar gives one credential to each verified eligible person, and campaign-specific serial numbers let the collector reject repeated use. Auditable issuance, strong authentication, revocation for stolen credentials, and separation of registration from collection address the main risks. These controls prevent impersonation and duplicate counting; authentication verifies identity, not motive. An eligible saboteur may sign in order to push the list over the threshold and expose everyone else, so strategic sabotage remains a separate design risk.

\paragraph{Custody, collusion, and availability}
A centralized custodian can leak names, invent or discard entries, suppress a successful list, or yield to coercion. Distributed trustees, signed submission receipts, a log whose old entries cannot be silently rewritten, and a quorum release rule divide those powers. Distribution creates two opposing risks. A sufficiently large group of trustees may cooperate to open records early, while too few available trustees may prevent release after success. Choosing trustees from institutions with different interests, setting a quorum that tolerates some failures, protecting key shares, and precommitting legal duties and penalties reduce both risks. Collusion-deterrent escrow protocols show how the technical design can also make early cooperation against the rules less attractive to trustees \citep*{mangipudiCollusionDeterrentThresholdInformation2023}.

\paragraph{Software, keys, and governance}
A system built from sound cryptographic tools can still fail because of compromised devices, poor key storage, code defects, or an administrator's power to change the software. A participant's device might reveal her action or trick her into signing a substituted statement; a bug might reject valid submissions or apply the threshold incorrectly. Conservative software design, independent security audits, open-source review, hardware-backed or multiparty key custody, and clear recovery procedures can reduce these risks. The statement, roster rule, threshold, deadline, and release policy should be cryptographically tied to the contract identifier and should not be alterable by one administrator after collection begins. Decentralized-finance smart contracts held about \$150 billion in total value as of April 2022, showing that related infrastructure operates at large scale \citep{wernerSoKDecentralizedFinance2022}. Attacks on these systems have also exposed recurring failures in design, governance, dependencies, and implementation \citep*{rezaeiSoKRootCause2025}. Those failures provide a concrete list of risks for system design and audit.

\paragraph{Metadata and public observability}
Encryption hides the contents of a submission, not necessarily its \emph{metadata}: where it came from, when it was sent, or the fact that it exists. If every encrypted submission is a public transaction, observers may learn the interim count and perhaps link a transaction to a participant even though they cannot read the encrypted contents. Grouping submissions into batches, routing them through intermediaries, delaying their recording, and collecting them privately rather than on a public chain can reduce those disclosures. A system concerned only with failed-name privacy may tolerate a public encrypted count. Implementing the article's stronger observation $\varnothing$ requires that the exposure-cost audience also see no count, failure announcement, or evidence that the campaign was attempted. The technical architecture can protect names without assuming that every deployment hides the attempt itself.

Legal and institutional controls remain useful throughout. Contracts can penalize misconduct, audits can expose deviations from the release rule, and administrators can build reputational capital by operating transparent open-source systems. These safeguards complement cryptography. The distributed design greatly reduces the authority entrusted to any one party: it replaces trust in one custodian with narrower, auditable assumptions about credential issuance, software, logs, and a trustee quorum. No single person or organization receives readable access to submissions, unilateral control of the count, and unilateral release authority.

\subsection{Networks and Deployment}\label{app:implementation_networks}

Four networks matter for deployment, and they need not contain the same people or follow the same links. The \emph{recruitment network} determines which eligible people learn of the contract. The \emph{trust network} determines whether recipients believe the invitation and the custody arrangement. The \emph{exposure network} identifies the audience able to impose material costs after names become public. The \emph{observation network} determines whether outsiders learn that a campaign was attempted or failed.

Dense trusted groups can supply a plausible committed seed. An organizer can recruit a protected or already-public core through existing professional, organizational, or social ties before reaching more distant eligible participants. Bridges across departments or social circles determine who can be reached. In the model, these network features map into the seed $b(\theta)$, participating capacity $Y(\theta)$, and threshold reachability. Fragmented recruitment lowers capacity even when latent support is ample.

The exposure network answers the practical question of who can punish a signer. In an insular organization, supervisors or close peers may be the relevant audience; in a public campaign, employers, professional associations, or a wider political audience may matter. The homogeneous exposure benchmark applies when protection depends mainly on final coalition size. Network position, seniority, and subgroup membership instead map into the heterogeneous protection technology developed in the companion paper.

Finally, private recruitment and public attempt observability are separate design choices. Trusted invitations can spread through the recruitment network while the outside exposure audience sees no campaign. Public advertising or a visible progress counter may improve reach, but it also turns a failed campaign into a public event and can reveal how close the threshold came. The benchmark therefore describes a specific configuration: private recruitment of a credible seed, enough potential participation to reach the threshold in the state being evaluated, a seed that can clear it in favorable states, and an information policy that keeps failed lists and attempts from the exposure audience.

Implementation burden and distrust can raise the signing friction $k$ by making participation harder or less attractive. Premature or partial disclosure is more serious: it exposes signers before the coalition is large enough to protect them and violates the institution analyzed in the paper. A working system must provide the eligibility, custody, verification, and release functions described above under assumptions suited to the attacks and failures it may face. Existing institutional and cryptographic tools make such a system plausible. The security of a particular deployment depends on how those tools are combined and operated.

\ifSubfilesClassLoaded{%
  \bibliographystyle{aea}
  \bibliography{conditional_disclosure}
}{ }

\end{document}
